# Supplementary material for: GRID: Scene-Graph-based Instruction-driven Robotic Task Planning
Source: arXiv:2309.07726 source file (2024-03-11)
Supplement: Supplementary file 1 [file appendix.tex]

% \section*{Appendix}

\subsection{Dataset Details}\label{Sec-Dataset_Details}

\begin{table}[h]
        \centering
	\begin{tabular}{ lp{5cm} }
		\hline
		\textbf{Relationship} & \textbf{Definition} \\
		\hline
		in & target object is in source object \\
		
		on & target object is on top of source object \\

		beside & target object and source object are in the same parent object, 
		the Euclidean distance between their 6DoF positions are less than one metre apart,
		target object is the closest object to the source object, while they do not have 'in' or 'on' relationships.
		\\
		
		grasp & target object is grasped by the source object \\
		\hline
	\end{tabular}
	\caption{The type of edges in the graph and their definitions. More other relationships can be added if it is needed to be used in more complex scenes.}
	\label{tab edge definition}
\end{table}

\begin{table*}[t]
    \centering
	\begin{tabular}{ llp{0.2\textwidth} }
        \hline
        \textbf{Task Type} & \textbf{Instruction Example} & \textbf{Subtasks Example} \\
        \hline
        \multirow{3}{0.2\textwidth}{Move-Place-Finish} 
        &\multirow{3}{0.3\textwidth}{Please move to the green dining table and place the object there}
        & move 22 (dining table) \\
        & & place to 22 (dining table) \\
        & & finish 0 (floor)\\
        
        \hline
        %  pick place\_to finish
        \multirow{3}{0.2\textwidth}{Pick-Place-Finish}
        &\multirow{3}{0.3\textwidth}{Please pick up the tea cup and place it on the green dining table.}
        & pick 45 (tea cup)\\
        && place to 22 (dining table)\\
        && finish 0 (floor)\\
        \hline

        \multirow{3}{0.2\textwidth}{Move-Pick-Finish}
        &\multirow{3}{0.3\textwidth}{Can you please go to tea cup and pick it up?}
        & move 45 (tea cup)\\
        && pick 45 (tea cup)\\
        && finish 0 (floor)\\
        \hline

        \multirow{4}{0.2\textwidth}{Move-Pick-Place-Finish}
        &\multirow{4}{0.3\textwidth}{Move to tea cup, pick it up, then place it on the dining table.}
        & move 45 (tea cup)\\
        && pick 45 (tea cup)\\
        && place to 22 (dining table)\\
        && finish 0 (floor)\\
        \hline

        \multirow{4}{0.2\textwidth}{Pick-Move-Place-Finish}
        & \multirow{4}{0.3\textwidth}{Pick up the tea cup. Then, proceed towards dining table. Once there, place it.}
        & pick 45 (tea cup)\\
        && move 22 (dining table)\\
        && place to 22 (dining table)\\
        && finish 0 (floor)\\
        \hline

        \multirow{5}{0.2\textwidth}{Pick-Move-Place-Move-Finish}
        &\multirow{5}{0.3\textwidth}{Please pick up the tea cup, move to the dining table, place it there, then proceed to the kitchen.}
        & pick 45 (tea cup) \\
        && move 22 (dining table)\\
        && place to 22 (dining table)\\
        && move 1 (kitchen)\\
        && finish 0 (floor)\\
        \hline

        \multirow{5}{0.2\textwidth}{Move-Pick-Place-Move-Finish}
        &\multirow{5}{0.3\textwidth}{Could you first move to the tea cup, pick it up, then take it to the dining table and place it there? After doing so, please proceed to the kitchen.}
        & move 45 (tea cup)\\
        && pick 45 (tea cup)\\
        && place to 22 (dining table)\\
        && move 1 (kitchen)\\
        && finish 0 (floor)\\
        \hline

        \multirow{5}{0.2\textwidth}{Pick-Move-Place-Move-Pick-Finish}
        &\multirow{5}{0.3\textwidth}{Please pick up the tea cup, move to the dining table, and place it there. Then proceed to the kitchen.}
        & pick 45 (tea cup)\\
        && move dining table 11\\
        && place to 45 (tea cup)\\
        && move 1 (kitchen)\\
        && finish 0 (floor)\\
        \hline

        \multirow{6}{0.2\textwidth}{Place-Move-Pick-Move-Place-Finish}
        &\multirow{6}{0.3\textwidth}{Put the object at the dining table. Then go to the tea cup and pick it up. At the end, go to kitchen table and put it there.}
        & place to 22 (dining table)\\
        && move 45 (tea cup)\\
        && pick 45 (tea cup)\\
        && move 7 (kitchen table)\\
        && place to 7 (kitchen table)\\
        && finish 0 (floor)\\
        \hline

        % Revolute open/close
        \multirow{5}{0.2\textwidth}{Move-RevOpen-Pick-RevClose-Finish}
        &\multirow{5}{0.3\textwidth}{Please proceed to the fridge, open it up, grab the apple inside, then make sure to close it.}
        & move 35 (fridge)\\
        && revolute open 35 (fridge)\\
        && pick apple 30\\
        && revolute close 35 (fridge)\\
        && finish 0 (floor)\\
        \hline
        % longitudinal open/close
        \multirow{5}{0.2\textwidth}{Move-LongOpen-Pick-LongClose-Finish}
        &\multirow{5}{0.3\textwidth}{Please proceed to the draw, open it up, grab the tea cup inside, then make sure to close it.}
        & move 9 (draw)\\
        && longitudinal open 9 (draw)\\
        && pick 45 (tea cup)\\
        && longitudinal close 9 (draw)\\
        && finish 0 (floor)\\
        \hline

        \multirow{5}{0.2\textwidth}{Move-RevOpen-Place-RevClose-Finish}
        &\multirow{5}{0.3\textwidth}{Head to the fridge, open it up, place the object inside, and then secure it shut.}
        & move 35 (fridge)\\
        && revolute open 35 (fridge)\\
        && place to 35 (fridge)\\
        && revolute close 35 (fridge)\\
        && finish 0 (floor)\\
        \hline
        \multirow{5}{0.2\textwidth}{Move-LongOpen-Place-LongClose-Finish}
        &\multirow{5}{0.3\textwidth}{Head to the draw, open it up, place the object inside, and then secure it shut.}
        & move 9 (draw)\\
        && longitudinal open 9 (draw)\\
        && place to 9 (draw)\\
        && longitudinal close 9 (draw)\\
        && finish 0 (floor)\\
        \hline

        \multirow{6}{0.2\textwidth}{Move-RevOpen-Place-Revclose-Move-Finish}
        &\multirow{6}{0.3\textwidth}{Please head to the fridge, open it, place the object inside, close it, then proceed to the kitchen.}
        & move 35 (fridge)\\
        && revolute open 35 (fridge)\\
        && place to 35 (fridge)\\
        && revolute close 35 (fridge)\\
        && move 1 (kitchen)\\
        && finish 0 (floor)\\
        \hline
        \multirow{6}{0.2\textwidth}{Move-LongOpen-Place-Longclose-Move-Finish}
        &\multirow{6}{0.3\textwidth}{Please head to the draw, open it, place the object inside, close it, then proceed to the kitchen.}
        & move 9 (draw)\\
        && longitudinal open 9 (draw)\\
        && place to 9 (draw)\\
        && longitudinal close 9 (draw)\\
        && move 1 (kitchen)\\
        && finish 0 (floor)\\
        \hline
        % Removed task type of length 7
        % \multirow{7}{0.2\textwidth}{move open pick close move place\_to finish}
        % &\multirow{7}{0.3\textwidth}{Please move to the fridge, open it, pick up an tea cup inside, close it, then move to the dining table and place it there.}
        % & move 35 (fridge)\\
        % && revolute open 35 (fridge)\\
        % && pick 45 (tea cup)\\
        % && revolute close 35 (fridge)\\
        % && move 22 (dining table)\\
        % && place to 22 (dining table)\\
        % && finish 0 (floor)\\
        % \hline
	\end{tabular}
    \caption{Instruction-subtask examples.}\label{tab-instruction-subtask-examples}
\end{table*}

\subsection{Training Details}\label{Sec-Training_Details}
GRID is implemented on the PyTorch toolbox. 
It is optimized via AdamW and the peak learning rate is 1e-4 and decays according to a one cycle learning rate schedule with diversity factor 10 and final diversity factor 1e-4.
We train our models 500 iterations with a batch size of 240 in total on two NVIDIA RTX 4090 GPUs.
The loss weights are $\alpha = 5, \beta = 25$.
The L1 and L2 regularization strength are $\gamma = 0.2, \delta = 0.8$.

\subsection{GPT-4 evaluation settings}\label{Sec-GPT_Settings}

We follow the method of Chalvatzaki \emph{et al.} \cite{chalvatzaki_learning_2023} to evaluate the subtask and task accuracy of GPT-4 in robotic manipulation planning tasks on our datasets.
We provide a GPT-4 evaluation example for the robotic manipulation planning task, as shown in Tab. \ref{tab-GPT_Prompt}:

\subsection{Simulation Experiment Details}\label{Sec-Simulation_Details}
Unity offers the ROS-TCP Connector communication framework, which enables seamless publishing of standard ROS2 topic messages from the Unity platform through ROS-TCP Connector. Additionally, Unity can subscribe to external messages using this framework. 

\begin{figure}[t]
    \centering
    \includegraphics[width=\columnwidth]{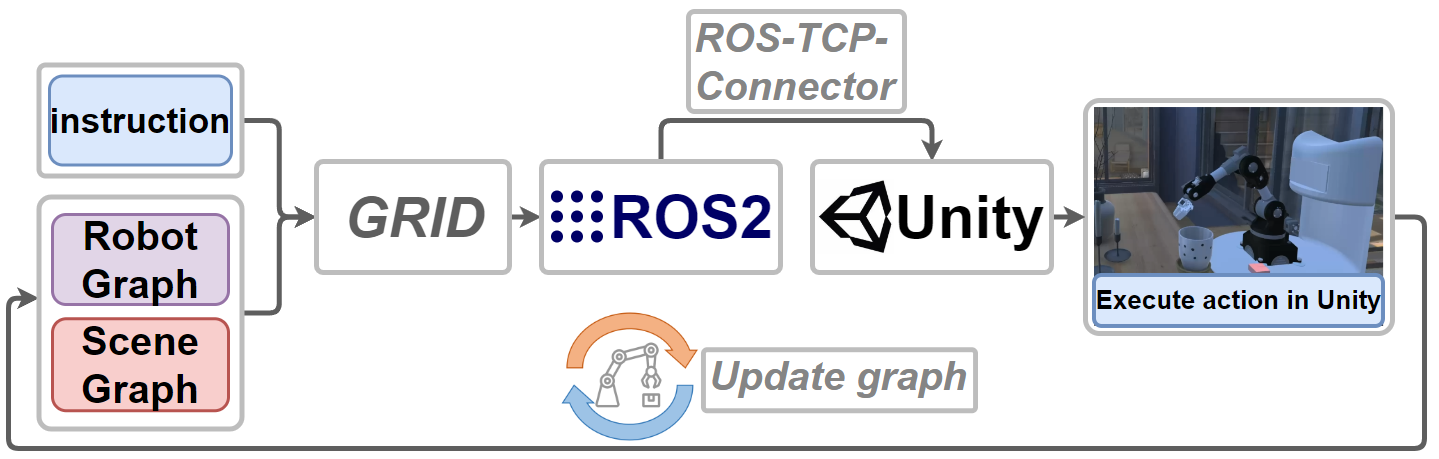}
    \caption{Simulation experimental process design.}
    \vspace{-10pt}
    \label{Simulation experimental process design.}
    % \label{fig-First_Pic}
\end{figure}

\begin{table*}[t]
    \centering
    \begin{tabular}{|p{0.95\textwidth}|}
        \hline
        \\
        \#Role:
        \\\quad You are an instruction planning model for a mobile grasping robot, your aim is to break down high-level instruction into subtasks for the robot to execute. 
        \\\#Output Restriction: 
        \\\quad Your output is in a form of \textless action\textgreater \textless operating object name\textgreater \textless operating object id\textgreater , where \textless action\textgreater is one of the actions in 
        ['move', 'pick', 'finish', 'place\_to', 'LongOpen', 'LongClose', 'RevOpen', 'RevClose'], 

        The meaning of the actions are:
        \\\quad move: controls the robot movement, the target object is the location where the robot will be moved to.
        \\\quad pick: controls the robot arm, the target object is the object which the robot should pick up.
        \\\quad finish: Showing that the high-level instruction task is completed. The target object does not matter thus the object prediction can be anything.
        \\\quad place\_to: controls the robot arm, the target object is the location where the robot will place the grasping object to.
        \\\quad LongOpen: controls the robot arm to perform a longitudinal open movement on an object, like a sliding drawer or dresser.
        \\\quad LongClose: controls the robot arm to perform a longitudinal close movement on an object, like a sliding drawer or dresser.
        \\\quad RevOpen: controls the robot arm to perform a revolute open movement on an object, like a hinged door or cabinet.
        \\\quad RevClose: controls the robot arm to perform a revolute close movement on an object, like a hinged door or cabinet.

        The \textless operating object name\textgreater  \textless operating object id\textgreater are the object and ids given in the prompt \#Scene.
        Specially, When robot think the task has already reached completion, or the robot should wait for further instruction, output: finish floor 0.

        \\\#Scene:
        \\\quad The current scene has objects with ids: \textless \texttt{scene graph nodes description}\textgreater 
        The relationships between objects in the scenes are: \textless \texttt{scene graph edges description}\textgreater 
        \\\#Robot:
        \\\quad The objects and object ids around the robot are: \textless \texttt{robot graph edges description}\textgreater 
        The relationships between objects around the robot are: \textless \texttt{robot graph edges description}\textgreater 
        \\\#Instruction:
        \textless \texttt{instruction}\textgreater 
        \\\#Task: Please tell me what is the current subtask the robot should perform according to the scene and robot status.
        
        \\\#Example1:
        \\\quad input: 
            \\\quad\#Scene:
            \\\quad\quad The current scene has objects with ids: floor 0, dining room 1, black dining table 2, purple display shelves 3, bathroom 4, brown vanity sink 5
            \\\quad\quad The relationships between objects in the scenes are: dining room 1 is in floor 0, dining table 2 is in dining room 1, display shelves 3 is in dining room 1, bathroom 4 is in floor 0, vanity sink 5 is in bathroom 4
            \\\quad\#Robot:
            \\\quad\quad The objects and object ids around the robot are: robot 0, brown pen 2.
            \\\quad\quad The relationships between objects around the robot are: pen 2 is grasped by robot 0.
            \\\quad\#Instruction:
            Your goal is to get the object to the purple display shelves.
            \\\quad\#Task: Please tell me what is the current subtask the robot should perform according to the scene and robot status.
            \\\quad\#Think: Because I do not know where I am, so I should first move to purple display shelves. So output: move purple display shelves 3.
            
        \\\#Example2:
        \\\quad input: 
            \\\quad\#Scene:
            \\\quad\quad The current scene has objects with ids: floor 0, dining room 1, black dining table 2, purple display shelves 3, bathroom 4, brown vanity sink 5, brown pen 6
            \\\quad\quad The relationships between objects in the scenes are: dining room 1 is in floor 0, dining table 2 is in dining room 1, display shelves 3 is in dining room 1, bathroom 4 is in floor 0, vanity sink 5 is in bathroom 4, brown pen 6 is on display shelves 3
            \\\quad\#Robot:
            \\\quad\quad The objects and object ids around the robot are: robot 0, purple display shelves 3.
            \\\quad\quad The relationships between objects around the robot are: pen 2 is grasped by robot 0.
            \\\quad\#Instruction:
            Your goal is to get the object to the purple display shelves.
            \\\quad\#Task: Please tell me what is the current subtask the robot should perform according to the scene and robot status.
            \\\quad\#Think: Because I no longer have anything grasped in my manipulators, and I am approaching another object, this indicates that I have already completed the instruction to place the object. So output: finish floor 0.

        \\
        \hline
    \end{tabular}
    \caption{The template of prompt and role being sent to ChatGPT4, we fill in the instruction and serialized graph descriptions to get an response from chatGPT4 API.}
    \label{tab-GPT_Prompt}
\end{table*}

\textbf{Graph Generation and Update.}
In our simulation experiments, we utilize Unity to process the scene and robot states, generating Scene Graph and Robot Graph information. This information is then published to the local area network space as ROS2 standard topic types. The topic (/SGRG-info) serves as the input for the Scene Graph and Robot Graph components of the GRID network. The GRID network outputs its results through the ROS2 topic (/GRID-output), which Unity subscribes to. Based on the instructions received from the topic, Unity controls robot motion accordingly.

The execution of instructions by the robot leads to changes in the Scene Graph and Robot Graph states. The updated Scene Graph and Robot Graph information then serves as new inputs for the network, initiating a continuous feedback loop, as described above.

we devised an intelligent mapping mechanism, where we cleverly mapped the directory structure of the hierarchy's parent and child classes to the tree structure of the graph. During scene initialization and detection of directory structure changes, we transform the hierarchy directory into a graph representation and publish it via the ROS2 topic.

To ensure the correspondence between robot-object interactions and the updates in Scene Graph and Robot Graph, we incorporated fixed target points into the design. As objects in the scene move to or from these target points, the hierarchy's parent-child relationships change, triggering the script responsible for the transformation of the directory structure. The overall process is illustrated in Fig. \ref{fig-The process of generating and updating Graphs in Untiy}.

\begin{figure*}[t]
    \centering
    \includegraphics[width=\textwidth]{figure/Simulation/Method for Generating and Updating Unity Scene Maps.png}% nz:文件名最好别有空格？
    \caption{The process of generating and updating scene graph in Unity.}
    \vspace{-10pt}
    \label{fig-The process of generating and updating Graphs in Untiy}
\end{figure*}

\subsection{Real World Deployment Details}\label{Sec-Real_Details}
Unlike the simulation experiment, the update of real scene images and robot images is contingent upon the real sensors' updates. The scene knowledge is constructed into scene graph by scene graph generation (SGG) methods, wherein the pose of objects can be obtained by a 6DoF pose estimation model \cite{armeni_3d_2019, kim_3-d_2020, rosinol_3d_2020, zhu_hierarchical_2021}.
% TODO 补充实验图，SGG内容加上
\begin{figure}[t]
    \centering
    \includegraphics[width=\columnwidth]{figure/Real experiments/real_exp_structure.png}% nz:文件名最好别有空格？
    \caption{The process of generating and updating Graphs in real world.}
    \vspace{-10pt}
    \label{The process of generating and updating Graphs in real world}
\end{figure}
